# Supplementary material for: Belief-based Generation of Argumentative Claims
Source: arXiv:2101.09765 source file (2021-01-26)
Supplement: Supplementary file 1 [file eacl21-belief-based-claim-generation-appendix-1.tex]

\section{Detailed Table of Automatic Evaluation}
\label{sec:appendix-1}
In Table \ref{table-automatic-evaluation-full}, we show the accuracy of the linear stance classifier when trained on claims generated by all approaches and tested against all the 48 big issues. Due to space restrictions, we abbreviated the big issues as follows: (AB) Abortion, (DL) Drug Legalization, GW (Global Warming), (DP) Death Penalty, (EP) Environmental Protection, (MM) Medical Marijuana, (AA) Affirmative Action, (AR) Animal Rights, (BO) Barack Obama, (Cap) Capitalism, (CU) Civil Unions, (EC) Electoral College, (ET) Estate Tax, (EU) European Union, , (Euth) Euthanasia, (FR) Federal Reserve, (FT) Flat Tax, (FreeT) Free Trade, (GWE) Global Warming Exists, (Glob) Globalization, (GS) Gold Standard, (GR) Gun Rights, (HS) Homeschooling, (IC) Internet Censorship, (IIW) Iran-Iraq War, (LU) Labor Union, (LP) Legalized Prostitution, (M\&M) Medicaid \& Medicare, (MM) Medical Marijuana, (MI) Military Intervention, (MW) Minimum Wage, (NHC) National Health Care, (NRST) National Retail Sales Tax, (OM) Occupy Movement, (PT) Progressive Tax, (RP) Racial Profiling, (Red) Redistribution, (SP) Social Programs, (SS) Social Security, (Soc) Socialism, (StS) Stimulus Spending, (TL) Term Limits, (Tor) Torture, (UN) United Nations, (WA) War in Afghanistan, (WT) War on Terror, (Wel) Welfare.

\begin{table*}[h!]%
\centering%

\setlength{\tabcolsep}{6pt}%
\begin{tabular}{lrrrrrrrrrr}
\toprule
Approach & Ab & AA & AR & BO & BF & Cap & CU & DP & DL & EC\\
\midrule
GT          & 0.49	&0.46	&0.48	&0.52	&0.62	&0.44	&0.49	&0.59	&0.55	&0.42 \\
\midrule
S2S-baseline& 0.49	&0.46	&\bf 0.66	&0.52	&0.46	&0.53	&\bf 0.56	&0.48	&0.45	&\bf 0.54 \\
S2S-model   & 0.55	&0.5	&0.51	&0.59	&\bf 0.52	& 0.5	&0.5	& \bf 0.55	&0.45	&\bf 0.54  \\
LM-baseline & 0.48	&0.51	&0.55	&0.52	&0.46	&0.49	&0.48	&0.5	&0.49	&0.41  \\
LM-model    & \bf0.58	& \bf 0.6	&0.62	&\bf 0.6	&0.5	&\bf 0.58	&0.44	&0.53	& \bf 0.56	& \bf 0.54  \\
\midrule
\# Training instances & 1610	&1244	&1806	&1208	&1092	&1428	&1288	&1532	&1538	&1060 \\
\# Test instances & 350	&162	&120	&194	&280	&154	&142	&366	&316	&142 \\
\bottomrule

\toprule
Approach &EP	& ET	& EU	& Euth &FR	&FT	&FreeT	& GM	&GWE 	& Glob\\
\midrule
GT          & 0.55	&0.49	&0.54	&0.63	&0.49	&0.55	&0.54	&0.55	&0.55	&0.57 \\
\midrule
S2S-baseline& 0.51	&\bf 0.57	&0.48	&0.51	&0.51	&0.49	&0.46	&0.52	&0.51	&0.51 \\
S2S-model   & \bf 0.58	&0.45	&0.51	&0.42	&0.51	&0.49	&0.46	&0.45	&0.51	&0.46 \\
LM-baseline &  0.56	&0.45	& \bf 0.56	& \bf 0.54	&0.51	& \bf 0.56	&\bf 0.53	& \bf 0.54	&0.54	& \bf 0.52\\
LM-model    & \bf 0.58	&0.53	&0.49	&0.51	& \bf 0.55	&0.55	&0.47	&0.45	& \bf 0.61	&0.47 \\
\midrule
\# Training instances & 2196	&1032	&730	&1380	&622	&922	&1304	&2098	&1960	&882 \\
\# Test instances & 86	&152	&158	&152	&134	&176	&72	&196	&156	&136 \\
\bottomrule

\toprule
Approach & GS	& GR	&HS	&IC	&IIW	&LU	&LP &M\&M	& MM	& MI\\
\midrule
GT          & 0.52	&0.48	&0.51	&0.55	&0.53	&0.51	&0.55	&0.49	&0.5	&0.5 \\
\midrule
S2S-baseline& 0.54	&0.55	&0.51	&0.41	&0.4	&0.41	&0.49	&0.44	&0.57	&0.54 \\
S2S-model   & 0.42	&0.48	&0.54	&0.49	&0.49	&0.4	&0.47	&0.55	&0.57	&0.49 \\
LM-baseline & 0.54	&0.49	&0.45	&\bf 0.51	& 0.63	&\bf 0.49	&\bf 0.6	&0.51	&0.51	&0.44 \\
LM-model    & \bf 0.57	& \bf 0.59	& \bf 0.58	&0.42	&\bf 0.66	&0.47	&0.52	&\bf 0.56	&\bf 0.58	&\bf 0.51 \\
\midrule
\# Training instances & 594	&1890	&1302	&1910	&1668	&1126	&1186	&1324	&2096	&910 \\
\# Test instances & 130	&182	&138	&98	&68	&146	&230	&138	&138	&144 \\
\bottomrule

\toprule
Approach & MW	&NHC	&NRST	&OM	&PT	&RP	&Red	&SB	&SP	&SS\\
\midrule
GT          & 0.48	&0.54	&0.53	&0.43	&0.66	&0.46	&0.45	&0.53	&0.44	&0.51 \\
\midrule
S2S-baseline& 0.53	&0.53	&\bf 0.54	&0.46	&\bf 0.51	& \bf 0.61	&\bf 0.55	&0.53	&0.5	&0.45 \\
S2S-model   & 0.49	&0.56	&\bf 0.54	&\bf 0.54	&0.45	&0.47	&0.49	&\bf 0.53	& \bf 0.54	&0.55 \\
LM-baseline & 0.59	&0.57	&\bf 0.54	&0.43	&0.46	&0.54	&0.49	&0.45	&0.41	&0.48 \\
LM-model    & \bf 0.65	&\bf 0.62	&0.49	&0.53	&0.5	&0.55	&0.49	& \bf0.53	&0.51	& \bf0.56 \\
\midrule
\# Training instances & 1580	&1364	&802	&680	&800	&1728	&764	&1370	&1278	&1418 \\
\# Test instances & 172	&218	&168	&138	&178	&112	&144	&294	&114	&130\\
\bottomrule

\toprule
Approach & Soc	&SS	&TL	&Tor. &UN	&WA	&WT	&Wel.\\
\midrule
GT          & 0.59	&0.56	&0.55	&0.47	&0.54	&0.44	&0.54	&0.55 \\
\midrule
S2S-baseline& 0.5	&0.48	&0.5	&0.45	&0.57	&0.49	&0.47	&0.44 \\
S2S-model   & 0.48	&0.5	&\bf 0.54	&0.45	& \bf 0.62	&0.51	&\bf 0.52	& \bf 0.55 \\
LM-baseline & 0.47	&0.4	&0.41	&0.51	&0.59	&0.45	&\bf 0.52	&0.49 \\
LM-model    & \bf 0.59	& \bf 0.63	&0.49	& \bf 0.53	&0.58	&\bf 0.57	& \bf 0.52	&0.48 \\
\midrule
\# Training instances & 1100	&664	&1548	&1616	&1474	&1564	&1274	&1256 \\
\# Test instances & 174	&120	&112	&152	&160	&136	&252	&196\\
\bottomrule

\end{tabular}%
\caption{Accuracy achieved by a stance classifier trained on claims generated by the evaluated model}
\label{table-automatic-evaluation-full}%
\end{table*}

\newpage

\section{Manual Evaluation of big-issues}
In the following table, we show example words that were collected into the pro/con bag-of-words of \textit{Abortion}.
\begin{table}[h!]%
	\centering%
	\small
	
	\setlength{\tabcolsep}{4pt}%
	\begin{tabular}{lp{1cm}p{1cm}p{1cm}p{1cm}}
		\toprule
		& \bf Irrelevant & \multicolumn{3}{c}{\bf Relevant}\\
		\cmidrule(l@{0pt}r@{0pt}){2-2}\cmidrule(l@{5pt}r@{0pt}){3-5}
		Words & \bf c1 & \bf c2 & \bf c3 & \bf c4\&c5\\
		\midrule
		Pro & goes, homemade & murder, alive, illegal & aborted, procedures  & option, fetus, mother, right\\
		\midrule
		Con & getting, doubles & -- & delivery, rate, abort & contraception, conception, sanctity\\
		\bottomrule
	\end{tabular}%
	\caption{Example Pro/Con words for each category for \textit{Abortion} as a big issues}
	\label{table-bow-examples}%
\end{table}
