# Supplementary material for: Belief-based Generation of Argumentative Claims
Source: arXiv:2101.09765 source file (2021-01-26)
Supplement: Supplementary file 2 [file eacl21-belief-based-claim-generation-appendix-automatic-eval.tex]

\begin{table*}[h!]%
\centering%

\setlength{\tabcolsep}{6pt}%
\begin{tabular}{lrrrrrrrrrr}
\toprule
Approach & Ab & AA & AR & BO & BF & Cap & CU & DP & DL & EC\\
\midrule
GT          & 0.49	&0.46	&0.48	&0.52	&0.62	&0.44	&0.49	&0.59	&0.55	&0.42 \\
\midrule
S2S-baseline& 0.49	&0.46	&\bf 0.66	&0.52	&0.46	&0.53	&\bf 0.56	&0.48	&0.45	&\bf 0.54 \\
S2S-model   & 0.55	&0.5	&0.51	&0.59	&\bf 0.52	& 0.5	&0.5	& \bf 0.55	&0.45	&\bf 0.54  \\
LM-baseline & 0.48	&0.51	&0.55	&0.52	&0.46	&0.49	&0.48	&0.5	&0.49	&0.41  \\
LM-model    & \bf0.58	& \bf 0.6	&0.62	&\bf 0.6	&0.5	&\bf 0.58	&0.44	&0.53	& \bf 0.56	& \bf 0.54  \\
\midrule
\# Training instances & 1610	&1244	&1806	&1208	&1092	&1428	&1288	&1532	&1538	&1060 \\
\# Test instances & 350	&162	&120	&194	&280	&154	&142	&366	&316	&142 \\
\bottomrule

\toprule
Approach &EP	& ET	& EU	& Euth &FR	&FT	&FreeT	& GM	&GWE 	& Glob\\
\midrule
GT          & 0.55	&0.49	&0.54	&0.63	&0.49	&0.55	&0.54	&0.55	&0.55	&0.57 \\
\midrule
S2S-baseline& 0.51	&\bf 0.57	&0.48	&0.51	&0.51	&0.49	&0.46	&0.52	&0.51	&0.51 \\
S2S-model   & \bf 0.58	&0.45	&0.51	&0.42	&0.51	&0.49	&0.46	&0.45	&0.51	&0.46 \\
LM-baseline &  0.56	&0.45	& \bf 0.56	& \bf 0.54	&0.51	& \bf 0.56	&\bf 0.53	& \bf 0.54	&0.54	& \bf 0.52\\
LM-model    & \bf 0.58	&0.53	&0.49	&0.51	& \bf 0.55	&0.55	&0.47	&0.45	& \bf 0.61	&0.47 \\
\midrule
\# Training instances & 2196	&1032	&730	&1380	&622	&922	&1304	&2098	&1960	&882 \\
\# Test instances & 86	&152	&158	&152	&134	&176	&72	&196	&156	&136 \\
\bottomrule

\toprule
Approach & GS	& GR	&HS	&IC	&IIW	&LU	&LP &M\&M	& MM	& MI\\
\midrule
GT          & 0.52	&0.48	&0.51	&0.55	&0.53	&0.51	&0.55	&0.49	&0.5	&0.5 \\
\midrule
S2S-baseline& 0.54	&0.55	&0.51	&0.41	&0.4	&0.41	&0.49	&0.44	&0.57	&0.54 \\
S2S-model   & 0.42	&0.48	&0.54	&0.49	&0.49	&0.4	&0.47	&0.55	&0.57	&0.49 \\
LM-baseline & 0.54	&0.49	&0.45	&\bf 0.51	& 0.63	&\bf 0.49	&\bf 0.6	&0.51	&0.51	&0.44 \\
LM-model    & \bf 0.57	& \bf 0.59	& \bf 0.58	&0.42	&\bf 0.66	&0.47	&0.52	&\bf 0.56	&\bf 0.58	&\bf 0.51 \\
\midrule
\# Training instances & 594	&1890	&1302	&1910	&1668	&1126	&1186	&1324	&2096	&910 \\
\# Test instances & 130	&182	&138	&98	&68	&146	&230	&138	&138	&144 \\
\bottomrule

\toprule
Approach & MW	&NHC	&NRST	&OM	&PT	&RP	&Red	&SB	&SP	&SS\\
\midrule
GT          & 0.48	&0.54	&0.53	&0.43	&0.66	&0.46	&0.45	&0.53	&0.44	&0.51 \\
\midrule
S2S-baseline& 0.53	&0.53	&\bf 0.54	&0.46	&\bf 0.51	& \bf 0.61	&\bf 0.55	&0.53	&0.5	&0.45 \\
S2S-model   & 0.49	&0.56	&\bf 0.54	&\bf 0.54	&0.45	&0.47	&0.49	&\bf 0.53	& \bf 0.54	&0.55 \\
LM-baseline & 0.59	&0.57	&\bf 0.54	&0.43	&0.46	&0.54	&0.49	&0.45	&0.41	&0.48 \\
LM-model    & \bf 0.65	&\bf 0.62	&0.49	&0.53	&0.5	&0.55	&0.49	& \bf0.53	&0.51	& \bf0.56 \\
\midrule
\# Training instances & 1580	&1364	&802	&680	&800	&1728	&764	&1370	&1278	&1418 \\
\# Test instances & 172	&218	&168	&138	&178	&112	&144	&294	&114	&130\\
\bottomrule

\toprule
Approach & Soc	&SS	&TL	&Tor. &UN	&WA	&WT	&Wel.\\
\midrule
GT          & 0.59	&0.56	&0.55	&0.47	&0.54	&0.44	&0.54	&0.55 \\
\midrule
S2S-baseline& 0.5	&0.48	&0.5	&0.45	&0.57	&0.49	&0.47	&0.44 \\
S2S-model   & 0.48	&0.5	&\bf 0.54	&0.45	& \bf 0.62	&0.51	&\bf 0.52	& \bf 0.55 \\
LM-baseline & 0.47	&0.4	&0.41	&0.51	&0.59	&0.45	&\bf 0.52	&0.49 \\
LM-model    & \bf 0.59	& \bf 0.63	&0.49	& \bf 0.53	&0.58	&\bf 0.57	& \bf 0.52	&0.48 \\
\midrule
\# Training instances & 1100	&664	&1548	&1616	&1474	&1564	&1274	&1256 \\
\# Test instances & 174	&120	&112	&152	&160	&136	&252	&196\\
\bottomrule

\end{tabular}%
\caption{Accuracy achieved by a stance classifier trained on claims generated by the evaluated model}
\label{table-automatic-evaluation-full}%
\end{table*}
